# Supplementary material for: Vertiport Navigation Requirements and Multisensor Architecture Considerations for Urban Air Mobility
Source: arXiv:2311.07487 source file (2023-11-13)
Supplement: Supplementary file 1 [file appendix_A.tex]

% An appendix contains supplementary information that is not an essential part of the text itself but which may be helpful in providing a more comprehensive understanding of the research problem or it is information that is too cumbersome to be included in the body of the paper.
